# Supplementary material for: Neural 3D Reconstruction in the Wild
Source: arXiv:2205.12955 source file (2022-05-25)
Supplement: Supplementary file 1 [file evaluation_supp.tex]

\newcolumntype{Y}{>{\centering\arraybackslash}X}
\newcolumntype{L}{>{\arraybackslash}X}
\begin{table}[t]
\centering
\setlength{\tabcolsep}{2.8pt}

\begin{tabular}{lllcccccccccccccccccc}
\toprule
Level  && BG  && LM   &&  PE  &&  PBA     \\ \midrule
Low    && 0.1 && 0.01 && 0.04 && 0.2 \\
Medium && 0.2 && 0.02 && 0.06 && 0.4 \\
High   && 0.3 && 0.03 && 0.08 && 0.6 \\
AUC-max    && 0.6 && 0.05  && 0.2  && 0.8 \\
\bottomrule
\end{tabular}
\caption{Values of evaluation thresholds in meters. \normalfont{We report the values of low, middle and high error thresholds used in the evaluation. AUC-max represents the maximum range of the curve used to calculate the AUC.}
}
\label{tab:error_thresh}
\end{table}
