# Supplementary material for: Neural 3D Reconstruction in the Wild
Source: arXiv:2205.12955 source file (2022-05-25)
Supplement: Supplementary file 2 [file num_images_supp.tex]

\begin{table*}[]
\setlength{\tabcolsep}{1.0pt}
 
\centering
		\setlength\tabcolsep{2pt}
\begin{tabular}{cccclccclccclcllll} 
\hline
\multirow{2}{*}{\begin{tabular}[c]{@{}c@{}}num\\images\end{tabular}} & \multicolumn{3}{c}{Low}                                                        &  & \multicolumn{3}{c}{Mid}                                                        &  & \multicolumn{3}{c}{High}                                                       &  & \multicolumn{3}{c}{AUC}                                    &  & \multicolumn{1}{c}{\multirow{2}{*}{Time}}  \\ 
\cline{2-4}\cline{6-8}\cline{10-12}\cline{14-16}
                                                                     & P                        & R                        & F                        &  & P                        & R                        & F                        &  & P                        & R                        & F                        &  & P                        & \multicolumn{1}{c}{R}                        & \multicolumn{1}{c}{F}    &  & \multicolumn{1}{c}{}                       \\ 
\hline
25\%                                                                  & 30.75                    & 31.38                    & 31.06                    &  & 61.99                    & 60.29                    & 61.13                    &  & 77.91                    & 76.56                    & 77.23                    &  & 3.20                     & 3.15                     & 3.17 &  & 14.10                                      \\
50\%                                                                  & 30.50                    & 33.30                    & 31.84                    &  & 62.43                    & 62.98                    & 62.70                    &  & 78.54                    & 79.48                    & 79.01                    &  & 3.22                     & 3.27                     & 3.24 &  & 14.23                                      \\
75\%                                                                  & 31.59                    & 34.58                    & 33.02                    &  & 63.03                    & 64.03                    & 63.52                    &  & 78.46                    & 79.12                    & 78.79                    &  & 3.23                     & \multicolumn{1}{r}{3.29} & 3.26 &  & 21.62                                      \\
100\%                                                                  & \multicolumn{1}{l}{\textbf{32.83}} & \multicolumn{1}{l}{\textbf{35.56}} & \multicolumn{1}{l}{\textbf{34.14}} &  & \multicolumn{1}{l}{\textbf{67.67}} & \multicolumn{1}{l}{\textbf{68.72}} & \multicolumn{1}{l}{\textbf{68.19}} &  & \multicolumn{1}{l}{\textbf{82.07}} & \multicolumn{1}{l}{\textbf{82.13}} & \multicolumn{1}{l}{\textbf{82.10}} &  & \multicolumn{1}{l}{\textbf{3.37}} & \textbf{3.40}                     & \textbf{3.38} &  & 22.42                                       \\
\hline
\end{tabular} 

\caption{\textbf{Effect of the number of images used for reconstruction}. \normalfont{More images lead to better reconstruction quality. However, training also takes more time}.}
\label{tab:num_images}
\end{table*}
