# Supplementary material for: Neural 3D Reconstruction in the Wild
Source: arXiv:2205.12955 source file (2022-05-25)
Supplement: Supplementary file 3 [file num_src_supp.tex]

\begin{table*}
\setlength{\tabcolsep}{1.0pt}
 
\centering
		\setlength\tabcolsep{2pt}
\begin{tabular}{cccclccclccclccl} 
\hline
\multirow{2}{*}{\begin{tabular}[c]{@{}c@{}}source\\ views\end{tabular}} & \multicolumn{3}{c}{Low} &  & \multicolumn{3}{c}{Mid} &  & \multicolumn{3}{c}{High} &  & \multicolumn{3}{c}{AUC}                 \\ 
\cline{2-4}\cline{6-8}\cline{10-12}\cline{14-16}
                                                                        & P     & R     & F       &  & P     & R     & F       &  & P     & R     & F        &  & P    & R    & \multicolumn{1}{c}{F}                         \\ 
\hline
20                                                                      & \textbf{23.37}  & 27.04          & 25.07          &  & \textbf{46.30}  & 42.72          & 44.44          &  & \textbf{63.78}  & 52.98          & 57.88         &  & \textbf{2.73} & 2.36          & 2.52          \\
40                                                                      & 23.02           & \textbf{31.11} & \textbf{26.46} &  & 45.72           & \textbf{48.84} & \textbf{47.23} &  & 62.35           & \textbf{61.02} & \textbf{61.68}&  & 2.67          & \textbf{2.71} & \textbf{2.68}              \\
80                                                                      & 20.43           & 28.46          & 23.78          &  & 42.95           & 46.03          & 44.44          &  & 61.32           & 57.17          & 59.17         &  & 2.61          & 2.56          & \multicolumn{1}{r}{2.57}  \\
\hline
\end{tabular}
\caption{\textbf{Vis-MVS results with different number of source images}.
}
\label{tab:src_views}
\end{table*}
