# Supplementary material for: Neural 3D Reconstruction in the Wild
Source: arXiv:2205.12955 source file (2022-05-25)
Supplement: Supplementary file 4 [file performance_supp.tex]

\newcolumntype{Y}{>{\centering\arraybackslash}X}
\newcolumntype{L}{>{\arraybackslash}X}
\begin{table}[t]
\centering
\setlength{\tabcolsep}{2.8pt}

\begin{tabularx}{0.61\columnwidth}{lllcccccccccccccccccc}
\toprule
Method &&  BG && LM &&PE && PBA     \\ \midrule
 NeRF-W && 37.8 && 43.5 && 39.0 && 89.6 \\
Vis-MVS && 13.7 && 9.4 && 19.8 && 48.0 \\
COLMAP && 21.4 && 47.3 && 31.4 && 197.6 \\
Ours \includegraphics[width=9pt]{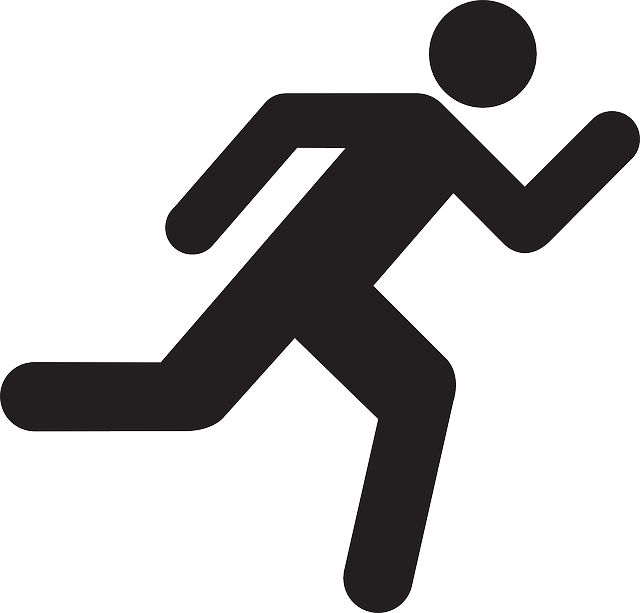}    && \textbf{9.7} && \textbf{7.5} && \textbf{11.5} && \textbf{14.3} \\
Ours && 30.7 && 22.4 && 20.7 && 26.0 \\
\bottomrule
\end{tabularx}
\caption{Training time of different methods measured in hours.
}
\label{tab:training_time}
\end{table}
