# Supplementary material for: Neural 3D Reconstruction in the Wild
Source: arXiv:2205.12955 source file (2022-05-25)
Supplement: Supplementary file 5 [file sfm_voxel_size_supp.tex]

\begin{table*}[h]
\setlength{\tabcolsep}{2.0pt}
 
\centering
		\setlength\tabcolsep{4pt}
\begin{tabular}{cccclccclccclccl} 
\hline
\multirow{2}{*}{\begin{tabular}[c]{@{}c@{}}sfm \\voxel\end{tabular}} & \multicolumn{3}{c}{Low} & \multicolumn{1}{c}{} & \multicolumn{3}{c}{Mid} &  & \multicolumn{3}{c}{High} & \multicolumn{1}{c}{} & \multicolumn{3}{c}{AUC}                 \\ 
\cline{2-4}\cline{6-8}\cline{10-12}\cline{14-16}
                                                                     & P     & R     & F       &                      & P     & R     & F       &  & P     & R     & F        &                      & P    & R    & \multicolumn{1}{c}{F}                         \\ 
\hline
x0.5                                                                 & 33.11 & \textbf{37.88} & 35.33   &                      & 65.81 & 68.34 & 67.05   &  & 80.61 & 81.95 & 81.27    &                      & 3.32 & \textbf{3.42} & 3.37                      \\
x2.0                                                                 & \textbf{34.51} & 37.67 & \textbf{36.02}   &                      & 64.55 & 65.25 & 64.90   &  & 79.70 & 79.10 & 79.40    &                      & 3.31 & 3.33 & 3.32                      \\
x1.0                                                                 & 32.83 & 35.56 & 34.14   &                      & \textbf{67.67} & \textbf{68.72} & \textbf{68.19}   &  & \textbf{82.07} & \textbf{82.13} & \textbf{82.10}    &                      & \textbf{3.37} & 3.40 & \multicolumn{1}{r}{\textbf{3.38}}  \\
\hline
\end{tabular}

\caption{\textbf{Effect of different SFM voxel sizes}. \normalfont{Doubling or halving the SFM voxel size has little effect on the reconstruction result. The proposed surfaced-guided sampling technique generates samples centered at surface position with a predefined range, which is irrelevant to initial SFM voxel size.}}
\label{tab:sfm_voxel_size}
\end{table*}
